# Supplementary material for: Sparse Attention Acceleration with Synergistic In-Memory Pruning and On-Chip Recomputation
Source: arXiv:2209.00606 source file (2022-09-01)
Supplement: Supplementary file 1 [file appendix.tex]

\onecolumn
\section*{Appendix}
\noindent{}We have adopted the suggested changes, fixed the typos, and justified the references in the revision. We have highlighted the changes in the paper in $\color{magenta}{magenta}$.

\setcounter{section}{0}

\section{Suggested Revision Summary}
\begin{enumpacked}
\item \niparagraph{Data Movement Overhead (Reviewer A) -- Communication between ReRAMs (Standard and Transposable) and between ReRAMs and On-chip Accelerator} $\rightarrow$ See paragraph ``\textit{Data movement cost analysis}'' in Section~\vref{para:datamove}.
\item \niparagraph{Breakdown of Benefits (Reviewer A, B)} $\rightarrow$ See Figure~\vref{fig:energy_saving_contribution} and its description for energy.

See added description in ''\textit{Performance and energy comparison}'' of \vref{subsec:perf_results} for speed-up.
\item \niparagraph{Details of \sys Simulator (Reviewer C)}$\rightarrow$ See paragraph ``\textit{\sys performance simulator}'' in Section \vref{para:perfsim}.
\item \niparagraph{Feed-Forward Computations and Improvements for \bench{BERT} and \bench{ViT} (Reviewer B, D)} $\rightarrow$ See paragraph ``\textit{End-to-End-Comparison-with-FFN-Support}'' in Section~\vref{para:ffn}.
\end{enumpacked}

\section{Clarifications}
\begin{enumpacked}
\item \niparagraph{Reviewer(A, C) --- Figure-7-Detail Overview of \sys} $\rightarrow$ See Figure~\vref{fig:overview} and revised Table~\vref{table:arch_config}.
\item \niparagraph{Reviewer(A) --- GOPs/s/J/mm$^2$} $\rightarrow$ See Table~\vref{table:comparison}.
\item \niparagraph{Reviewer(A, C) --- Spatial Locality Window Size} See Section~\vref{subsec:spatial}. 

\item \niparagraph{Reviewer(B) --- Figure-11-Speedup for Self-Attention} $\rightarrow$ Figure~\vref{fig:speedup} depicts the overall speedup of self-attention mechanism. We updated the captions of all the figures accordingly.

The analysis including feed-forward is analyzed in Section~\vref{para:ffn}.
\item \niparagraph{Reviewer(C) --- CORELET Explanation} $\rightarrow$ See Section~\vref{sec:hardware_arch}.
\item \niparagraph{Reviewer(A, C) --- Microarchitectural Details} $\rightarrow$ See Table~\vref{table:arch_config} and Table~\vref{table:perf_sim} with detailed description in Section~\vref{sec:memPrune}.
\item \niparagraph{Reviewer(C, D) --- Model Accuracy without On-Chip Recompute} $\rightarrow$ On-chip recompute is essential to preserve model accuracy. See Section~\ref{subsec:perf_results} and Figure~\vref{fig: accuracy}.
\item \niparagraph{Reviewer(E) --- ReRAM simulations} $\rightarrow$ We added a footnote in paragraph ``\textit{\sys hardware simulations}'' in Section~\vref{para:nvsim}.
\end{enumpacked}
